# Supplementary material for: It's All In the Teacher: Zero-Shot Quantization Brought Closer to the Teacher
Source: arXiv:2203.17008 source file (2022-04-01)
Supplement: Supplementary file 1 [file bakdds.tex]

Epoch	cifar10resnet20zqce	cifar10resnet20zqkl	cifar100resnet20zqce	cifar100resnet20zqkl	cifar10resnet56zqce	cifar10resnet56zqkl	cifar100resnet56zqce	cifar100resnet56zqkl	cifar10resnext29zqce	cifar10resnext29zqkl	cifar10wrn28zqce	cifar10wrn28zqkl	cifar100wrn28zqce	cifar100wrn28zqkl	cifar10wrn40zqce	cifar10wrn40zqkl	cifar100wrn40zqce	cifar100wrn40zqkl	cifar10resnet20kdce	cifar10resnet20kdkl	cifar100resnet20kdce	cifar100resnet20kdkl	cifar10resnet56kdce	cifar10resnet56kdkl	cifar100resnet56kdce	cifar100resnet56kdkl	cifar10resnext29kdce	cifar10resnext29kdkl	cifar10wrn28kdce	cifar10wrn28kdkl	cifar100wrn28kdce	cifar100wrn28kdkl	cifar10wrn40kdce	cifar10wrn40kdkl	cifar100wrn40kdce	cifar100wrn40kdkl
1	13.01113913	4.588234796	13.02412632	4.59278429	13.04422587	4.808716301	14.15742535	5.474554725	13.00306973	5.598150382	12.79937208	5.156916721	13.93590521	4.719260786	12.11825323	4.971098171	14.04356026	4.858224864	9.726872479	5.064584377	9.003076064	4.029402919	9.562876444	4.770418404	8.347616596	3.309315613	7.128266793	2.734240261	10.2704402	5.87981265	10.55643384	5.52059657	9.770400781	4.906079026	10.64407396	5.663725011
2	12.9986417	4.602396946	13.03232102	4.558648942	13.04293228	4.828152542	14.1763052	5.473635093	13.2446025	5.586561717	13.03713778	5.2799636	13.89694365	4.672615997	12.39151916	5.083932063	13.93860122	4.989450077	9.68419478	5.203713582	10.11685906	5.199265968	9.62245394	4.997170189	9.230134871	4.133144582	9.011320117	4.821589386	10.07319248	5.829416459	10.97158956	6.051601686	9.925875601	5.143002697	11.17388461	6.321463138
3	13.00955387	4.589107798	13.00961962	4.577820545	12.95731254	4.705816619	14.14698768	5.477440236	13.33569729	5.651281322	13.03291794	5.247355563	13.8414882	4.633626847	12.1849032	5.018516505	14.20178336	5.237544272	10.0161556	5.41903549	10.42890736	5.624807353	9.787894714	5.229738916	10.0155854	5.11709555	9.397951043	5.079935757	10.51712992	6.270096443	11.08385307	6.29116032	10.38565836	5.728771857	11.25804565	6.36321244
4	13.03089454	4.580836317	12.99491571	4.526318131	12.71140733	4.624632413	14.08418191	5.452784527	13.46263278	5.723079853	13.19756532	5.3674827	13.84825989	4.677841713	12.1289892	5.030466843	14.22684918	5.350333035	9.737535801	5.428595333	10.58795944	5.945358659	9.873286862	5.346673388	10.38400106	5.650831862	9.55372098	5.276221926	9.914776401	5.39509729	11.11687101	6.502090761	10.01033637	5.402443054	11.15797627	6.455336079
5	12.87173185	4.607716137	12.84664064	4.635479722	12.4747283	4.229480497	13.63793401	5.073190057	13.49014062	5.822232924	13.01006443	5.158863506	13.85821999	4.65551443	12.18954667	4.865055562	14.2617858	5.524630951	9.928739929	5.611104133	10.62098196	6.024523627	9.767309103	5.329836103	10.670404	6.016729203	10.02982988	5.948148439	10.08421027	5.828952024	11.20641557	6.48236383	9.889797286	5.041358878	11.14239577	6.446537653
6	13.08726771	5.068516045	13.04829814	5.00747956	12.27544587	4.059130574	13.73540003	5.280135245	13.35234454	5.658962259	12.90034262	4.989818855	13.89295475	4.659170639	11.95321581	4.742581093	14.33433717	5.598789388	10.00518649	5.592083786	10.66396541	6.087903271	9.927429766	5.390387084	10.73982166	6.246103516	10.29363301	6.088703571	9.96873508	5.737913646	11.0169668	6.218027416	9.900197527	5.128541249	11.10014591	6.451441726
7	13.21145853	5.323081436	13.16638918	5.326531594	12.35671921	4.103959413	13.79453579	5.521076952	13.48134168	5.644595941	12.60973977	4.911015746	13.83154362	4.68128918	12.04505111	4.780257003	14.33094463	5.705994821	9.743631495	5.543112738	10.874117	6.293347386	9.637009285	5.289912487	10.88929514	6.209118064	10.46651169	6.092154531	9.769216216	5.391409918	10.90605554	6.131642153	9.75643178	4.87800188	11.12656769	6.404882795
8	13.38021403	5.623777826	13.39830718	5.72826363	12.21638491	4.01943302	13.86898401	5.738254617	13.35790363	5.585322022	12.78707991	4.96553232	13.87342673	4.683355054	12.21382099	4.643689238	14.37092843	5.767951967	9.655510946	5.314571042	10.7744217	6.212326752	9.994342108	5.544465819	10.69017375	6.123806171	10.24789434	6.039244225	9.829902952	5.599854756	10.98864949	6.088007756	9.906609255	5.049869702	10.98418814	6.169284811
9	13.51136034	5.797756726	13.50044801	5.938442104	12.32948092	4.046898925	13.95427447	5.998020263	13.35822076	5.531476595	12.36700912	4.900045805	13.8572714	4.678106593	12.04232589	4.522480028	14.42538415	5.808302338	10.09787542	5.68857178	10.8166896	6.296322871	9.932069212	5.357811698	10.8898371	6.268181466	10.31564263	6.178917453	9.891683886	5.629991648	11.1744747	6.511114968	9.920580453	4.976529327	11.28698369	6.499371009
10	13.58584944	6.037417672	13.6464205	6.130208828	12.27295876	3.980362464	13.99035766	6.111814995	13.3202742	5.503318785	12.53500376	4.882447573	13.88783089	4.656535178	11.99889162	4.544642004	14.46171124	5.882293133	9.883301249	5.480070732	10.95203101	6.45104404	9.690481701	5.381023691	10.84320517	6.379428738	10.19887798	5.978643685	9.596382511	5.257008088	11.05553965	6.202301316	9.740985699	4.834301418	11.04181912	6.36812512
11	13.62616691	6.089223192	13.73002132	6.309057012	12.14799767	3.988379934	14.04498704	6.234644776	13.13627119	5.429146102	12.61101879	4.854007317	13.8619867	4.68412822	12.13977253	4.509723617	14.44695242	5.959867612	9.786847199	5.630912959	10.75070563	6.382447865	9.871693693	5.471662772	10.80291297	6.203501317	10.12457851	6.008591769	9.750729239	5.373376026	11.11366574	6.359480272	9.534423938	4.745148231	11.15934702	6.551022419
12	13.70489497	6.183429979	13.6909623	6.267927717	12.32786925	4.03402762	14.06503211	6.311117556	13.23103186	5.460238937	12.65692169	4.822240743	13.84715099	4.665081563	12.18593005	4.513347617	14.5082625	6.045946992	9.870305942	5.683447929	10.81494902	6.23034573	10.28841074	5.614927204	10.98262284	6.560095191	10.34445664	6.286143399	9.663660761	5.245928167	11.12641405	6.387952594	9.766819802	4.918169999	10.90748229	6.143059663
13	13.71954042	6.27751039	13.81989142	6.390769294	12.27686226	4.015946991	14.14401415	6.375895796	13.20123016	5.409979896	12.55830274	4.754946207	13.88361078	4.67161916	11.96747863	4.477412183	14.48814541	6.057049364	10.26755655	5.816169773	10.86488618	6.454025589	9.978222812	5.644819509	11.28296891	6.982637623	10.19769001	6.219991307	9.919089311	5.541107943	11.27688074	6.345235517	10.0454866	5.091977876	11.20929809	6.573426226
14	13.70433873	6.283260525	13.83336798	6.421863713	12.25878831	3.966800946	14.2223826	6.493012094	13.01753198	5.385409767	12.58494497	4.802970026	13.83572877	4.680486655	11.91486272	4.420533349	14.50596812	6.081826144	9.825155912	5.622139752	11.08336889	6.688376911	9.999823755	5.679874229	11.01003625	6.511008356	10.63779858	6.529154086	9.98804578	5.502561207	11.26332106	6.439642613	10.05705542	5.020782275	11.19856213	6.501583317
15	13.76617828	6.347818945	13.81533637	6.421762024	12.19815318	3.958176971	14.15505703	6.49223048	13.14589946	5.363468004	12.61606367	4.830563521	13.82771141	4.648072282	12.11742266	4.423524895	14.49743248	6.148972731	9.923708249	5.573731076	10.78339427	6.246593607	9.719115678	5.454893681	10.9071637	6.45086912	10.52260841	6.526876095	9.811254149	5.624679106	11.30484016	6.425963292	10.00772766	5.053426661	11.2268949	6.504924585
16	13.75768601	6.307342999	13.80419048	6.421360099	12.25894442	3.966197086	14.20420399	6.496311315	13.1859239	5.372699782	12.38631668	4.804725603	13.82293055	4.656002658	11.9340174	4.42206016	14.58629328	6.132771387	10.13894471	5.685785155	10.74723189	6.22296175	10.27585591	5.575783195	11.1103054	6.474370361	10.48494039	6.397891131	10.19255972	5.634767786	11.27700274	6.505790907	9.944347885	5.007872832	11.34120002	6.546347824
17	13.73814994	6.285168782	13.78116811	6.39685934	12.27302903	3.981976886	14.22357037	6.519026384	13.16551624	5.328584959	12.72173138	4.800649872	13.83813946	4.662251972	12.02432666	4.407624719	14.55105446	6.150626357	9.745415101	5.431356474	10.745972	6.180175226	9.909326362	5.556665399	11.27420383	6.724294525	10.74577387	6.789259262	10.16829952	5.772473555	11.54015659	6.636119565	10.04610251	5.149590587	11.34280978	6.489282115
18	13.67466723	6.253195349	13.76904007	6.399838892	12.23062912	3.91363088	14.17054332	6.595342429	13.12688624	5.298680593	12.50366854	4.726465769	13.86001357	4.658953293	11.96699167	4.476111738	14.56444856	6.160573188	10.12289243	5.757577957	10.66297241	6.099590849	10.06555391	5.560991063	11.0288997	6.541633646	10.80526858	6.65999432	10.21105059	5.824572753	11.39933187	6.52879356	9.782944737	4.888877477	11.44611298	6.492357052
19	13.65898732	6.254125822	13.77820014	6.380005872	12.23284308	3.889852931	14.15598461	6.507744381	13.10082598	5.288049147	12.32889765	4.762174072	13.83475713	4.659148217	11.85144932	4.444693854	14.55756967	6.19247754	9.850759266	5.619855848	11.04033214	6.575220795	9.845708499	5.602467502	11.08971761	6.668054781	10.63530245	6.658578404	10.38079588	5.668830418	11.59183871	6.649743887	10.26355111	5.279271224	11.37928621	6.898826391
20	13.60999981	6.181425582	13.78113205	6.341583132	12.26481371	3.943302106	14.15925142	6.545331125	13.12063306	5.295565166	12.34121776	4.7458012	13.82458596	4.677562521	11.87053435	4.47344449	14.58738452	6.224925337	10.40498899	6.053161454	10.99729586	6.596791886	9.797800309	5.694562452	11.09311127	6.63033498	10.59317586	6.531617387	9.799861526	5.491743164	11.70227636	6.660148747	10.05843238	5.226163397	11.31816647	6.561097926
21	13.55653515	6.1077705	13.70307424	6.324614616	12.21635115	3.916545383	14.23738147	6.568118134	13.19628174	5.279767948	12.48701037	4.743726109	13.92053568	4.978102729	11.96936482	4.490953763	14.58234388	6.227308731	9.964099946	5.722654224	10.67656707	6.102268799	9.637987044	5.451134004	11.08231489	6.680385867	10.68259623	6.576921675	9.784138653	5.431095726	11.53245689	6.734772842	9.941001695	5.15573341	11.36096605	6.75974005
22	13.61100308	6.144665009	13.73548325	6.257198859	12.18529691	3.869243013	14.23129626	6.548089023	13.11900918	5.268578318	12.63813216	4.795011834	13.95223406	5.151614274	12.00585586	4.512349166	14.67116508	6.20663159	9.878305415	5.76560199	10.80058938	6.286992322	9.913753832	5.844220697	10.98305796	6.518724714	10.538139	6.439661624	9.758672925	5.479959923	11.49633993	6.805267742	10.06139853	5.224985543	11.52929733	6.786259731
23	13.60844761	6.054652384	13.6738927	6.226788032	12.21734423	3.92238319	14.18138893	6.470267392	12.97247496	5.24198126	12.51419085	4.739588016	14.03252854	5.285986462	11.68361446	4.409479475	14.69317162	6.266790611	10.01723847	5.78850625	10.84163151	6.410301535	9.702144912	5.701772728	11.02803645	6.504737062	10.67508181	6.663899677	10.31703358	5.890849193	11.56396074	6.620555005	10.09230787	5.164254444	11.58454341	6.907231648
24	13.55411786	6.066183408	13.57635409	6.209799572	12.2442988	3.930547306	14.18351481	6.476439283	13.08138624	5.226509847	12.46255131	4.738622911	14.0937666	5.427319906	11.85977986	4.442003589	14.63306447	6.2677223	9.671889974	5.518547496	11.0716698	6.73648466	9.82548629	5.663133534	11.11612254	6.573281249	10.69830365	6.583574814	9.923113399	5.5895876	11.59131957	6.467445939	9.947968056	5.053616411	11.42988265	6.669460458
25	13.47755404	5.951786658	13.6464118	6.125716409	12.25097269	3.86234416	14.18411972	6.467357591	13.12088286	5.189179317	12.3570209	4.708331378	14.10189378	5.537720457	11.68808962	4.451142527	14.61575227	6.286000214	9.77489249	5.6326363	10.94224358	6.42562197	10.08072946	5.748624347	11.12257427	6.626005754	11.28346429	6.991859394	10.25308573	5.963422319	11.68358702	6.571301609	9.907308474	4.952438581	11.33913619	6.54395174
26	13.45206549	5.8915334	13.5497822	6.089683787	12.15831353	3.871787983	14.15816155	6.465282788	13.07419048	5.209139209	12.60248185	4.705199821	14.12613405	5.553491996	11.75268013	4.431749965	14.66694594	6.266078112	9.794957218	5.611877802	11.15314741	6.933755046	9.957750382	5.68341414	11.02484826	6.515879939	10.7366845	6.618477796	10.01549392	5.505541794	11.53254333	6.5800956	10.05552991	5.152982656	11.68337838	6.839737983
27	13.42765448	5.868418235	13.5787274	6.087119104	12.20323767	3.874129336	14.14074993	6.406471175	13.02341237	5.215736194	12.26453202	4.750600883	14.15809808	5.611209911	11.75553266	4.388422818	14.68177366	6.284889203	10.03231209	5.774909494	10.99058024	6.50372327	9.697406338	5.55759423	11.03256115	6.741048196	10.64151558	6.609484181	10.03152223	5.587250648	11.39478489	6.323779414	10.08510631	5.072962045	11.58617858	6.854862372
28	13.48884116	5.891570733	13.51977893	6.088993662	12.18689246	3.88018883	14.22279447	6.434815065	13.0709662	5.2405197	12.47716631	4.718610971	14.16130895	5.666451858	11.87608664	4.4474501	14.71477526	6.279670337	9.61603862	5.43063497	10.77502156	6.452897435	9.721304304	5.644013764	11.26285317	6.739392262	10.54598919	6.495111528	10.18449797	5.624548812	11.67918797	6.809184272	9.873011296	5.020696495	11.60114512	6.910769568
29	13.41476853	5.860702528	13.51615315	6.053691797	12.10148462	3.815681612	14.11816256	6.405559325	13.03577043	5.229578281	12.17674949	4.695985905	14.17841022	5.714656117	11.9636619	4.498035748	14.64003831	6.290909234	9.781668243	5.638449927	10.98602284	6.614807668	9.956017552	5.690602359	11.20750136	6.821669947	10.55408911	6.590578985	10.1945739	5.810862261	11.72476536	6.846177028	10.44517776	5.554608675	11.57990612	6.610634687
30	13.43682933	5.808673869	13.4683127	5.949755989	12.20442503	3.799730936	14.08675791	6.358966415	13.05393448	5.216923434	12.41286696	4.727034224	14.23387881	5.763269252	11.84892706	4.470514533	14.69160941	6.300226361	9.877434765	5.618191405	10.82663354	6.495607453	10.17548088	5.875133784	11.01298439	6.475565485	10.3873176	6.445193336	10.25134537	5.988093464	11.79858701	6.933153732	10.16076767	5.365317441	11.38364365	6.537050471
31	13.36646	5.78754533	13.47518898	5.95768903	12.14345664	3.867212645	14.10208709	6.38793987	12.97299484	5.194632916	12.25517115	4.649622493	14.24295636	5.817332062	11.70783055	4.393435403	14.71458085	6.261670065	9.862933783	5.676676188	10.81356657	6.367296753	9.771224177	5.5583143	11.10643437	6.67309799	10.61490801	6.72548364	9.972780105	5.627330958	11.6020405	6.700215708	9.961469972	5.173013913	11.47358104	6.606079184
32	13.3104159	5.790398017	13.43881187	5.904255901	12.02415938	3.817059924	14.12200414	6.311820778	13.01244394	5.170866623	12.33152844	4.713535427	14.16966327	5.817567981	11.90418232	4.391226991	14.70059548	6.27750836	9.669336703	5.615257882	10.91197774	6.460546617	9.825391463	5.630832901	11.11324988	6.422455623	10.44789588	6.456264989	9.900467945	5.626366824	11.66954416	6.48105652	10.39794323	5.368100179	11.4617345	6.678130956
33	13.37920544	5.746391275	13.44006722	5.89529466	12.1506456	3.846343152	14.12725354	6.305073842	12.91053711	5.145188918	12.31918947	4.670134543	14.21287103	5.830936061	11.96264808	4.448942733	14.72051916	6.25773463	9.854537317	5.675989498	10.70306607	6.222087838	9.643651912	5.523116164	11.12693234	6.646405373	10.3367466	6.541077898	10.07908989	5.635219134	11.63572593	6.973813496	10.19293753	5.48207578	11.42328538	6.59446463
34	13.36759193	5.712547073	13.41908077	5.84700052	12.16409695	3.832107394	14.14317053	6.285937983	12.9672508	5.201959442	12.38620389	4.749011227	14.31618886	5.87737727	11.76100297	4.375210096	14.8157935	6.263723064	10.0754832	5.762144094	10.90515396	6.417873605	9.985564016	5.693002659	11.07471237	6.72873329	10.75964047	6.766051899	10.26688979	5.885160631	11.72947428	6.744504384	10.11080623	5.161481553	11.50389261	6.564637468
35	13.31209112	5.75251317	13.38450645	5.780602352	12.2145749	3.829325615	14.08449258	6.245650927	12.99925986	5.154790299	12.37403843	4.724084347	14.3280732	5.907724022	11.90885781	4.410799147	14.74859415	6.253596775	9.692135802	5.535271489	10.95371188	6.407731185	9.935965615	5.636724166	11.04905564	6.48486557	10.40368462	6.596031271	10.12829206	5.67892468	11.57079276	6.67062595	10.15985567	5.249896966	11.70787514	6.983221313
36	13.32988101	5.662562837	13.35524275	5.805208229	12.19778048	3.831237287	14.05317078	6.231106327	12.8467552	5.110983872	12.32832613	4.736067267	14.2834702	5.926286296	11.76934037	4.440418157	14.65200308	6.261176303	9.933434278	5.785392662	11.03205868	6.630697212	9.815243465	5.673648076	11.05986741	6.637195642	10.43572241	6.520011736	10.00941188	5.862592522	11.51579011	6.643629857	10.13115695	5.317861075	11.6998978	6.788918332
37	13.22640271	5.615932365	13.39093963	5.747509623	12.18756189	3.811237561	13.9909706	6.171946036	12.86970525	5.113866273	12.49296862	4.752405012	14.28041083	5.92502579	11.9028942	4.438056294	14.76847909	6.265985099	9.846592623	5.580859487	11.05823453	6.654814843	10.03698753	5.867295728	11.40442522	6.973818897	10.53008871	6.655398066	10.42084711	5.875790391	11.98943547	7.268920213	10.0066106	5.068283111	11.57137393	6.839810701
38	13.25457784	5.619515573	13.33269931	5.743930707	12.12614636	3.809586759	13.99908935	6.192033877	12.9674457	5.179804609	12.32441141	4.741247891	14.28148515	5.95146118	11.61036269	4.388074092	14.72655039	6.233661295	9.938096002	5.631911307	11.11135425	6.738898851	10.1332738	5.795414916	11.24001245	6.711634154	10.58797915	6.66827737	10.23293145	5.996101847	11.6650937	6.678069048	10.02142351	5.28342129	11.61149982	6.652993899
39	13.23806487	5.563277457	13.33280191	5.723369554	12.06414925	3.791672591	14.01017718	6.145101177	12.85232528	5.100524382	12.39519118	4.739258589	14.36955766	5.964976551	11.80535455	4.402176804	14.71509472	6.209515569	10.09272205	5.601759217	11.08682101	6.70478668	10.27958714	5.777990523	11.28529101	6.770144568	10.71232976	6.745952407	10.20931406	5.810255313	11.98606774	6.84585749	10.08187316	5.35190156	11.69335022	6.811648105
40	13.16483331	5.544362579	13.30934734	5.662589818	12.11067522	3.792780483	14.02270292	6.111588404	12.98701148	5.15701113	12.56131663	4.743934956	14.34541253	5.929178468	11.88689095	4.397844843	14.75210805	6.192227844	9.687376096	5.562712881	11.02829778	6.694902474	10.05699005	5.801844432	11.18274722	6.759087138	10.59133762	6.694878216	10.09895628	5.611008374	11.83708283	6.943701299	10.0460626	5.129324482	11.6369428	6.896040045
41	13.21347811	5.564213556	13.31815647	5.663341375	12.09648236	3.827781579	14.00021923	6.154976323	12.97477223	5.171652182	12.19366215	4.68998741	14.26415568	5.952776406	11.8718707	4.399184672	14.74169395	6.21880268	9.742476568	5.758101875	10.97634692	6.558301165	10.22479391	5.850157937	11.15726455	6.720279325	10.71777663	6.742796627	10.05183105	5.628521736	11.75129023	6.907783284	10.14018895	5.233719289	11.60372461	6.893577875
42	13.19799565	5.512524649	13.273664	5.66275595	12.02503004	3.787627263	13.95284517	6.112203624	13.09916361	5.16328211	12.38982742	4.710738583	14.36410224	5.966570228	11.70142302	4.428008471	14.68243783	6.208588004	10.08405938	5.812731032	11.03418965	6.537915059	9.927900081	5.542570703	11.1591469	6.626640806	10.72001546	6.820480509	10.23022809	5.707775292	11.58324129	6.843112968	9.95966464	5.084660927	11.6204389	6.804620205
43	13.15649258	5.483029641	13.23428585	5.634069245	12.11037197	3.794473417	13.94674919	6.105556234	13.00189172	5.131436599	12.3244321	4.662951338	14.34306494	5.993421652	11.72567832	4.334723059	14.70256374	6.178191684	9.701613816	5.526697747	11.01819176	6.638558692	9.950597711	5.593051846	11.17821493	6.78684234	10.59752113	6.697057046	10.06362761	5.609445127	12.1092742	7.024786508	9.947520702	5.120035466	11.56350744	6.955993815
44	13.17028725	5.479710041	13.29349764	5.611847194	12.04976328	3.718506425	14.00013918	6.076880506	13.01721984	5.16918897	12.14603275	4.600062326	14.35948037	5.945084858	11.68000695	4.329629721	14.73597482	6.165543841	9.708559145	5.670214041	11.12038416	6.647664592	10.05676148	5.925945466	11.19176709	6.758469703	10.70913226	6.628707621	10.04591981	5.688517496	11.70136292	6.782636448	10.16070876	5.248889442	11.65306625	6.910402801
45	13.21268788	5.473261271	13.24559888	5.613770366	12.11899953	3.819663714	14.03029883	6.050498524	12.94606096	5.146292826	12.59770007	4.683312228	14.38875097	5.943158513	11.89087678	4.387679342	14.57226018	6.148560979	9.815424203	5.557878402	11.07985702	6.569737053	9.777519368	5.532912769	11.26754641	6.742630723	11.04468071	6.848105059	9.923598771	5.625154179	11.83256436	6.920345143	10.3815483	5.458426587	11.74418471	6.95846846
46	13.15385996	5.436516393	13.192054	5.604626777	12.13173824	3.794005282	13.98437048	6.03626177	12.84973879	5.129069333	12.39338795	4.658741745	14.38926067	5.978204101	11.91631718	4.323442697	14.55596817	6.147160835	10.2632932	6.046777693	10.89611548	6.409900122	9.911662466	5.705140934	11.22844714	6.686632145	10.68724672	6.688168497	10.39243729	5.949158861	11.74267033	6.932453117	10.04525529	5.091498452	11.63747647	6.956968095
47	13.17086522	5.419518008	13.24544767	5.537241922	12.18555867	3.798646843	13.96323722	6.009689772	12.90646094	5.108779326	12.39723233	4.63634014	14.40687533	5.968149958	11.69999256	4.317723889	14.6045168	6.130809983	9.908372673	5.718567972	10.98103009	6.433715096	9.911893779	5.851523881	11.25888612	6.636037421	10.68650475	6.693328985	9.973729545	5.654607532	11.75691867	6.852353631	9.786270406	4.925390711	11.65331727	6.635116173
48	13.08361611	5.463981012	13.19211666	5.496253248	12.05516056	3.759852301	13.93716724	6.03927654	13.0045875	5.169676015	12.30947084	4.586071456	14.4307774	5.97360734	11.6286296	4.377403206	14.67768615	6.129517741	10.27324839	5.838276594	11.09613022	6.804794129	9.973615768	5.724726895	11.13685131	6.684066822	10.40390376	6.600695894	10.06161059	5.638421395	11.79294308	6.83441507	10.3064779	5.337532551	11.77505967	6.73601249
49	13.01963221	5.39066174	13.20731074	5.50411711	12.02238158	3.772874002	13.93562738	5.984461651	12.90257171	5.123155182	12.35225455	4.665008882	14.36482824	5.939217533	11.77218145	4.377254994	14.60961732	6.086159357	10.03344909	5.752542321	11.06272579	6.616135357	9.921297055	5.677131159	11.1052369	6.677612137	10.66987758	6.700930677	10.42306544	5.853259147	11.86799737	6.790233658	10.00507293	5.288468736	11.74277723	6.804995606
50	13.0885637	5.411521838	13.18023873	5.528943744	11.98365431	3.747985871	13.92738345	5.960532266	12.96427425	5.135987042	12.58825155	4.679484982	14.36738742	5.953009881	11.75304902	4.346150047	14.68189849	6.127545398	10.07814657	5.723758476	11.15018388	6.776068377	10.55291047	6.190570898	11.36264993	6.981947631	10.87911355	6.738378337	10.3070221	5.917955893	12.05233863	7.113305375	10.19946856	5.169373846	11.58364491	6.714093157
51	13.12673426	5.374538342	13.14135994	5.512970241	12.12446151	3.811238496	13.94095631	5.971912776	12.95318073	5.12514764	12.37069892	4.70468393	14.3732381	5.925969351	11.50712582	4.303442178	14.65108825	6.10640705	10.56712237	6.043750721	10.96400624	6.622188876	10.27187028	5.695547022	11.30780504	6.833695378	10.51159261	6.654835247	10.03248877	5.842818519	11.9319661	7.033397149	10.42881613	5.452672297	11.55990339	6.729604252
52	13.05261158	5.409033411	13.1629313	5.450046357	12.18754394	3.771333118	13.92113452	5.946168668	12.96137013	5.118903826	12.49629334	4.695830567	14.32145024	5.941598492	11.61722953	4.318246371	14.55821965	6.074404836	10.22631136	5.924466772	11.02532477	6.535639853	10.11551702	5.830552391	11.28631878	6.842868379	10.85883923	6.911618674	10.02699684	5.694930285	11.85374173	7.174156507	10.68615519	5.695715757	11.66603314	7.040004854
53	13.03865451	5.342241729	13.12633409	5.418995865	12.14492911	3.723303862	13.89826601	5.941145537	12.89437021	5.079017615	12.22422983	4.593767419	14.38070185	5.914817302	11.6296907	4.290050549	14.67447419	6.104588634	9.591694102	5.57468241	11.0169688	6.642731043	9.859949959	5.654836884	11.20636802	6.575290946	10.82138909	6.912358974	10.08113191	5.839741244	11.92372101	7.017946337	10.03974201	5.321239648	11.81193325	7.09622451
54	13.15570805	5.321706622	13.15523522	5.393292458	12.09221486	3.779699242	13.96780713	5.965737986	12.87251223	5.078029641	12.48368669	4.624529966	14.38618053	5.936046007	11.58551474	4.32828938	14.58676878	6.110045643	9.602734723	5.52216389	11.11828468	6.629550176	9.819857122	5.52066752	11.26223832	6.635438988	10.69251805	6.732501318	10.06156081	5.567831021	11.92291645	6.891000368	10.40397093	5.369623584	11.79971543	7.101160631
55	13.06307373	5.332203104	13.12253535	5.380700539	12.0827582	3.799138643	13.93431373	5.961507794	12.89980595	5.090032217	12.24475201	4.701393195	14.39069923	5.944982954	11.7465243	4.317726578	14.67446682	6.082086045	10.1166003	5.882429707	10.96945697	6.52540883	10.11404229	5.670378973	11.30205967	6.755949133	10.75022391	6.670678666	10.36679702	5.820236525	11.85008001	6.967448803	10.10707798	5.170464213	11.83312752	7.027863296
56	13.06746851	5.314240075	13.12905525	5.365086383	12.06612694	3.847829247	13.90924166	5.949907805	12.92221559	5.127567685	12.35060413	4.66791796	14.37310764	5.938973163	11.55989833	4.269435969	14.71724235	6.074143805	9.849105279	5.784653483	11.05199719	6.606293208	9.936819715	5.746722656	11.13923722	6.689116071	10.83797614	6.775589219	9.98121715	5.601036716	11.95961362	6.899953427	9.89289592	5.131192553	11.82433065	7.022853829
57	13.05310554	5.309494227	13.12011628	5.407454163	12.11968564	3.802100383	13.90209753	5.922886446	13.03291995	5.062538637	12.41268328	4.684140983	14.42837243	5.954866073	11.49572879	4.307367489	14.62636224	6.060819829	9.904846855	5.557126059	10.97071371	6.635517474	9.969154338	5.783469351	11.37090087	6.953491269	10.95428634	6.921150991	10.01701799	5.687190286	11.93891985	6.95630587	10.00290473	5.296615067	11.65153521	6.702299659
58	13.06714798	5.311437837	13.10785183	5.371857	12.15060202	3.793365853	13.908005	5.89324097	13.00448944	5.116000375	12.26203596	4.667808946	14.43076971	5.925011316	11.5278378	4.262197789	14.68691128	6.04547947	9.969784643	5.688845494	11.10840377	6.806990322	9.716122089	5.489241114	11.38379221	6.846826076	10.54691268	6.707946144	10.77688452	6.248086335	11.94162879	7.000832404	10.20995418	5.483787039	11.77017241	7.066015461
59	12.99851323	5.296364011	13.07131836	5.352022141	12.13047042	3.749351937	13.86189533	5.902700005	12.90867037	5.104568388	12.29110099	4.640627303	14.36997451	5.946782579	11.4883378	4.234435851	14.59793422	6.039613849	9.890695717	5.665883947	10.92370649	6.521992095	10.0037173	5.784625448	11.52329746	7.056527662	10.46638181	6.707585881	9.771933701	5.713877412	11.97792863	7.25424929	10.35092818	5.31248151	11.85901695	7.204835578
60	13.03549938	5.255502341	13.08490639	5.329775129	12.02119893	3.762276693	13.8843089	5.863543008	12.80055445	5.066310352	12.20960226	4.618475224	14.36037163	5.935284963	11.58134393	4.166731344	14.60011438	6.030825869	10.03551554	5.931905301	11.09908308	6.830638647	9.902200273	5.583901251	11.36537063	6.592237257	10.82969878	7.071371777	10.22275001	5.781065922	11.89517024	7.158548347	10.25525077	5.386061995	11.79392005	6.986266827
61	13.0808897	5.248804848	13.08569301	5.361193468	12.17644444	3.809736338	13.83317974	5.831291571	12.97126451	5.110354972	12.42676044	4.654680114	14.39443407	5.880536496	11.49176688	4.226216507	14.54837652	6.009880384	9.71622594	5.657391625	11.11569871	6.706371927	9.800853646	5.794004817	11.36450303	6.870817276	10.77597365	6.905677336	9.871544511	5.668327561	11.92473682	7.290727884	10.06511371	5.269862835	11.62742749	6.83367216
62	12.99264254	5.220614227	13.10196263	5.335109172	12.1416193	3.699375767	13.83589691	5.856380919	13.00611511	5.128456887	12.44342443	4.72804804	14.42108587	5.906235448	11.6727704	4.200697632	14.71715813	6.027722455	10.21021601	5.816092308	11.00959893	6.523566561	10.42016963	6.051908637	11.08840979	6.502159973	10.84512443	6.927191838	10.26008793	5.853252969	11.99133634	7.053157927	10.42143409	5.512836915	11.76034955	6.993941367
63	13.00962634	5.230308667	13.06604894	5.305972294	11.99480356	3.75962423	13.80099192	5.816631246	12.96757742	5.141135286	12.40492523	4.695525412	14.40907034	5.91592563	11.50265352	4.200576077	14.65595578	6.002837049	10.10416342	5.908275124	10.88512098	6.463532448	9.986858823	5.700574762	11.39302103	6.782419167	10.86315788	6.931656036	10.09942008	5.695644706	11.96205674	7.20108213	10.15119159	5.163781899	11.87792459	7.197768049
64	12.98099038	5.26086396	13.08826495	5.2624923	12.11874915	3.751793709	13.80308781	5.800933231	12.96239228	5.133373381	12.42102283	4.679799754	14.31785474	5.906657727	11.55534903	4.22110304	14.5471805	6.038888339	10.00767114	5.724615944	11.04931133	6.615907904	10.05161193	5.766674791	11.35671548	6.732285923	10.73814408	6.812789484	9.897793688	5.60809438	11.9781769	6.987549572	10.08379382	5.365065847	11.72269547	6.720742514
65	12.93484225	5.204494987	13.04008738	5.291741188	12.16436867	3.742017081	13.85976787	5.831929409	13.0611292	5.100237623	12.42310141	4.716640715	14.39154988	5.903508098	11.51750884	4.23954249	14.63826684	5.989183524	10.34565471	5.969053562	11.13817221	6.742311326	10.34675484	5.781671822	11.14109469	6.70220911	10.84816017	6.913337641	9.92656033	5.657534246	11.91196607	6.997818982	10.18140494	5.294792407	11.68692354	6.96541076
66	13.03283869	5.240884437	13.05059689	5.255395174	12.00945799	3.725295504	13.79238637	5.802096864	12.85687931	5.109899536	12.31911344	4.612717666	14.3403225	5.878229971	11.75801389	4.227613321	14.65324997	5.998955814	10.5762293	6.227983068	10.96075405	6.551766051	9.901335848	5.655634576	11.32943922	6.900508481	10.52973555	6.607228994	10.14420504	5.884619732	11.90896364	6.932983887	9.815008674	5.235245726	11.60239901	6.860595398
67	12.96614756	5.223515159	13.06135535	5.291484071	12.10323266	3.754748884	13.76286826	5.783750347	13.03850997	5.100881822	12.38863077	4.695603063	14.36034462	5.856853047	11.50164169	4.215796246	14.63176794	5.977587827	10.23416481	5.89064126	11.03690378	6.72898081	10.53796681	5.874531415	11.69851264	6.914018093	10.64466267	6.503912807	10.2941786	5.76709519	11.99015259	6.940601288	10.17750833	5.298328665	11.67252849	6.936414384
68	12.920859	5.199827942	13.04243147	5.229816978	12.15603387	3.724826935	13.78156949	5.782260447	12.8219174	5.106392401	12.51838959	4.682786334	14.34913212	5.885243824	11.58863373	4.204274915	14.51342857	5.955749541	10.07736329	5.690354315	10.77441074	6.224529564	9.932987851	5.72599694	11.3816462	6.959037458	10.82814112	6.775143068	10.03935542	5.67274035	12.01227707	6.956119613	10.1428564	5.212495155	11.71666385	6.971120159
69	12.96506842	5.199398065	13.01186323	5.216286778	12.0914848	3.679755744	13.8427248	5.789447823	12.99002856	5.11053508	12.36954821	4.664916362	14.35636775	5.874575215	11.64528261	4.160706429	14.56046096	5.967544281	9.836844252	5.679410985	11.28108531	6.851290403	9.950831979	5.735353721	11.07176054	6.608078511	10.61408519	6.639661077	9.939419432	5.659431016	12.13204091	7.21421762	10.21168521	5.336563661	11.82405472	7.130406393
70	12.96232908	5.16703726	12.99929625	5.211559641	12.11654456	3.765163866	13.78181448	5.767740265	12.99708581	5.123457269	12.24484703	4.635151891	14.35856847	5.86788536	11.41463991	4.130741135	14.61171514	5.938530916	9.67448284	5.464927501	11.00506411	6.676587534	9.939621914	5.74875952	11.13945371	6.550925821	10.63618008	6.696408975	10.27675453	5.880200056	11.92498579	6.973951276	10.60633641	5.595690795	11.88475961	7.090299332
71	12.90416992	5.12353463	12.99888528	5.198453054	12.13861768	3.740518339	13.78213042	5.746172132	12.98373235	5.117153575	12.55979848	4.643806575	14.35892041	5.868774578	11.50297158	4.108287739	14.65803225	5.955255966	10.02195627	5.839067659	10.90206546	6.493350733	10.77124512	6.134707181	11.26941182	6.59445826	10.6948251	6.846899829	10.21084151	5.849843709	11.99125149	7.180824908	10.32214046	5.325158041	11.68068574	6.889265541
72	12.99082292	5.153570893	13.00430678	5.209960276	12.04545978	3.745869617	13.77454827	5.806423995	12.85923027	5.059142397	12.40785632	4.68375339	14.30599709	5.887024894	11.61535429	4.062917856	14.58135201	5.970757904	9.749215392	5.536416095	10.90971807	6.59356092	9.904025798	5.575693134	11.41050017	6.772792524	10.62775821	6.609835401	10.18846286	6.038610677	12.07095663	7.064092655	10.15596402	5.308751619	11.73174739	7.021538635
73	12.96505181	5.13718782	12.97393058	5.179606057	12.04564326	3.726113737	13.75158008	5.765716755	12.91255941	5.096897381	12.49644784	4.62773205	14.36843704	5.876514059	11.78249869	4.101618833	14.61619589	5.969856574	9.99178857	5.775474454	11.16081184	6.810864917	10.03812891	5.669087481	11.250394	6.809550432	10.45504511	6.471891738	10.1614486	5.835469596	12.02504721	7.386901009	10.38456673	5.518664293	11.86453821	7.170648755
74	12.91848897	5.115275957	13.01419882	5.203636767	12.12500524	3.729629066	13.79456884	5.751152958	12.86454678	5.086036288	12.61006108	4.666143236	14.33298614	5.839031841	11.82479347	4.102987141	14.71192782	5.912053822	10.03107281	5.716203141	11.19911713	6.863871148	9.858256041	5.680444569	11.26344963	6.674323939	10.75549625	6.807897386	10.08785332	5.843017598	11.97224349	7.234739604	9.871506232	5.164800963	12.10008305	7.467577227
75	12.91456008	5.121462086	12.98017131	5.153067683	12.16739143	3.788999006	13.82054725	5.750803647	12.73141894	5.080856957	12.43417079	4.695248653	14.38256917	5.858453833	11.63205757	4.110645804	14.58723385	5.911627637	9.924457465	5.611387726	11.07513334	6.635923308	10.19224443	5.934825043	11.30046499	6.734866714	10.559445	6.715965291	10.211818	5.675471933	12.05253777	7.133825428	10.15396632	5.240446694	12.00770654	7.059250853
76	12.90476644	5.081112168	13.0046048	5.185087147	12.13405716	3.748518758	13.77054601	5.741239949	12.84413143	5.086085238	12.56614911	4.716650231	14.35377692	5.853591706	11.66670046	4.157235469	14.51986795	5.914497064	9.821230278	5.735906521	11.42660676	7.079066058	10.1070061	5.71279122	11.30304831	6.779515671	11.16357853	6.963788073	9.8426788	5.630733675	11.82621661	6.843090296	9.928475483	5.161775962	11.82955326	7.143302737
77	12.86850935	5.105494608	12.98885045	5.194254202	12.04960807	3.732544059	13.82207961	5.7541424	12.84876696	5.054337525	12.4020461	4.702394976	14.34044692	5.82917124	11.62454667	4.155064875	14.57992981	5.923715694	9.734630646	5.563480498	10.94120354	6.407045726	10.54097154	6.160812137	11.27475779	6.756927059	10.74856239	6.574119941	10.41155508	5.911971296	12.14113602	7.382022767	10.06867903	5.207278225	11.78826104	6.893218007
78	12.88106229	5.058467828	13.00518162	5.121236951	12.15771654	3.763059958	13.77040464	5.6847487	12.88899066	5.031556089	12.39082456	4.660048906	14.35729501	5.859254574	11.72239386	4.103707785	14.65406113	5.947172985	9.693747667	5.55412348	10.95735743	6.543169011	9.843789995	5.581470972	11.28857892	6.746115817	10.71495347	6.780623613	10.05465711	5.767221034	12.2325865	7.388474608	9.941738706	5.139058187	11.84837217	7.210660161
79	12.92421316	5.095727303	12.95785335	5.151622828	12.28602638	3.827846007	13.78437664	5.709477968	12.88132998	5.11433287	12.315429	4.688760712	14.32478245	5.842342387	11.75970937	4.083484923	14.59109213	5.905870489	9.97145556	6.023435367	10.90811026	6.351572509	10.03735573	5.881876509	11.18215791	6.616430558	10.96281051	7.014456959	10.50073632	6.182445736	11.93413064	6.995859654	10.15430582	5.269225377	11.67761173	6.983536958
80	12.91368993	5.06702306	12.93670133	5.157270772	12.16692587	3.736401907	13.74885944	5.729996606	12.92622558	5.04961756	12.54539047	4.692939121	14.35033037	5.810999042	11.75156795	4.187333796	14.66809262	5.867839711	9.905914576	5.634531197	10.88754084	6.375865385	9.903088451	5.650187677	11.22595164	6.721687846	10.70084461	6.79300475	10.10934396	5.761598748	11.9639602	7.132947861	10.29986899	5.445699485	11.84125735	7.09460493
81	12.91037608	5.106453059	12.91538852	5.08625199	12.23570553	3.764050285	13.73382957	5.689428222	12.87612102	5.043397322	12.0210477	4.638097333	14.40296022	5.813762534	11.78486566	4.133950518	14.54660008	5.860453924	9.637974642	5.580144399	11.10882851	6.650667719	10.31705436	5.902769672	11.24288082	6.770990822	10.87228646	6.856783452	10.18231008	5.842099876	11.97845021	7.163269126	10.60328279	5.713916902	11.7421536	6.777561868
82	12.89375614	5.051826434	12.89830644	5.109418012	12.22050534	3.768771553	13.77359677	5.729866807	12.88918347	5.097219761	12.66572373	4.6942179	14.28768242	5.817064645	11.52475709	4.085038518	14.58708251	5.875737529	9.917633436	5.747950243	10.82209983	6.210621134	10.14220585	5.648148527	11.43359093	6.902221606	10.5371641	6.688874408	10.10544436	5.907390667	12.10881777	7.219206957	10.09922086	5.204169207	11.86275267	7.155165317
83	12.87337876	5.051791259	12.96130218	5.122838262	12.08537652	3.738116885	13.73972711	5.667882373	12.79802834	4.999769627	12.22817068	4.631463759	14.34549927	5.824115304	11.64353997	4.063249927	14.61135773	5.891679442	9.947290947	5.881748812	11.09281744	6.719333485	10.00110128	5.715852214	11.32741992	6.855511496	10.77057285	6.768819486	10.26833234	6.123346469	11.76326958	6.758844118	9.914452081	5.06749639	11.79818402	7.139004632
84	12.8924683	5.07392811	12.94129008	5.062162111	12.1530135	3.80834208	13.7078851	5.68004767	12.61683696	5.013428541	12.45319313	4.669640828	14.34096685	5.808219769	11.61212156	4.077030052	14.60565391	5.881459565	9.865715674	5.76276509	10.96817995	6.622049716	9.888586397	5.698437709	11.18937366	6.536109921	10.86223554	6.789426052	10.07113573	5.767296217	11.90382588	7.134756286	10.26860669	5.402918273	11.75389977	6.992995643
85	12.92933649	5.080340956	12.94602727	5.10643116	12.22494299	3.746265234	13.72691911	5.6761926	12.74363285	5.033112252	12.54260094	4.745619508	14.34681808	5.8049463	11.61524691	4.046800186	14.49066547	5.881134587	9.775643375	5.745979141	10.98018353	6.673534982	9.886628029	5.603070319	11.54485329	6.996598605	10.70214973	6.681130919	10.18332481	5.841540467	11.88613739	6.948643068	10.28506412	5.516840688	11.8676846	7.038290633
86	12.99054564	5.081309173	12.93710004	5.117970674	12.10850155	3.766912454	13.73317406	5.687538314	12.74867431	4.99432098	12.32547471	4.72010312	14.25270223	5.774278053	11.60736309	4.013562441	14.5672383	5.897303216	9.853745206	5.536847431	10.845745	6.380842527	10.10629381	5.563688757	11.19069482	6.628350159	10.78100173	6.81227942	9.887901198	5.714297991	11.97254301	7.128290571	10.08308652	5.31757341	11.84809883	7.081828175
87	12.91825438	5.069265552	12.90020108	5.080017403	12.18274206	3.82528261	13.74313152	5.688621179	12.76463899	5.007875989	12.25518725	4.705241068	14.37373962	5.788686339	11.77419666	4.033294281	14.54070021	5.874428976	9.866699755	5.770660863	10.77903341	6.308581452	9.927023875	5.67526186	11.0638483	6.56068581	10.65891434	6.832275926	10.40240476	5.888232435	12.07407994	7.204202052	9.899839579	4.972825692	12.26488963	7.369258608
88	12.91819042	5.09289054	12.90742719	5.111838854	12.13851161	3.734463902	13.66787163	5.637676666	12.77733056	5.013237814	12.34903885	4.652676829	14.41856417	5.74953986	11.82712503	4.075580205	14.61813766	5.86229132	9.80704084	5.478852899	10.85982416	6.258471965	10.41359798	5.995426434	11.28565006	6.983510195	10.86659442	6.883300018	10.28798768	5.839544596	12.05230741	7.196258996	9.946449913	5.149379117	12.11292362	7.292173524
89	12.85888656	5.031206307	12.91480466	5.030556679	12.16161727	3.754425557	13.77056414	5.681535367	12.83338972	5.02053509	12.43263353	4.627144594	14.35504802	5.756265323	11.62222332	3.994630369	14.61871277	5.85314635	9.898514525	5.774081959	11.09637654	6.398043646	10.13097098	5.809568302	11.27719258	6.976265583	10.45551404	6.610230016	10.33022931	5.991839981	12.01584978	6.941287075	10.03377727	5.194793122	11.92595289	7.387590661
90	12.88167282	5.06316333	12.90930188	5.066730221	12.19648541	3.724410008	13.77990484	5.721542729	12.93219369	5.040901442	12.38744131	4.687285504	14.32255927	5.753193957	11.7270863	4.085885357	14.6291031	5.874447885	9.998758792	5.802490168	11.13202206	6.897662852	9.921347264	5.88036727	11.3257199	6.774740435	10.99263691	7.089375493	10.09984144	5.65991733	12.08891403	7.216039374	10.1624788	5.232416401	11.56568335	6.630166462
91	12.83483217	4.992729848	12.91646644	5.074388878	12.16531363	3.765790188	13.68919441	5.682335854	12.84264578	5.022983485	12.20094969	4.649607944	14.24162257	5.760567485	11.49034447	4.008533698	14.54038895	5.875978636	9.765765431	5.607155611	10.91138822	6.408367146	10.03345715	5.776584597	11.23136341	6.74809804	10.65447761	6.715730119	9.936874313	5.583016923	12.13798451	7.31364077	10.15455373	5.287192317	11.92143824	7.244833066
92	12.87699646	5.048431576	12.89661192	5.068903559	12.24046775	3.789923542	13.74861765	5.69922744	12.7296267	4.99434995	12.16089898	4.597661532	14.35199664	5.727726729	11.62997551	4.040446333	14.57001685	5.855351061	10.02142692	5.813971546	11.23086901	6.916080114	10.02341825	5.831213344	11.30097801	6.812823076	10.86922062	6.79792784	10.25407558	5.841853601	12.02737486	7.197376319	10.15241752	5.414937956	11.81335998	6.973762926
93	12.90712086	5.01273373	12.86920003	5.03070018	12.08865655	3.743273567	13.73948395	5.655129834	12.82709164	4.991551234	12.40607135	4.641040981	14.35830036	5.734242202	11.62521252	4.110201914	14.59607632	5.877922765	9.797312047	5.607039607	10.8411779	6.515340825	10.30189715	5.739938127	11.17181034	6.715225317	10.84432569	6.861561496	10.12044992	5.714806136	12.08225325	7.248506432	10.53992288	5.522840295	11.84618963	7.074503338
94	12.86580891	4.985511243	12.88454645	5.017029971	11.98501866	3.739744188	13.7554696	5.620398918	12.85936467	5.02735579	12.26953425	4.686087865	14.36180227	5.73456766	11.44795344	3.990991944	14.56575263	5.849311462	9.852439991	5.70523193	10.85349402	6.478450015	10.35071897	5.99226591	11.25369878	6.86133962	10.95185549	7.028712435	10.13697094	5.804843758	12.00873123	7.043593775	10.43683458	5.555513159	11.83025947	6.967468843
95	12.88574302	4.984925734	12.8883629	5.022535611	12.16912339	3.815435721	13.76105862	5.690904415	12.71993537	5.022885298	12.44260708	4.636050667	14.40488184	5.745887985	11.63214578	3.988818788	14.62680979	5.888561265	9.94304017	5.622258714	11.11740008	6.763599203	9.993882129	5.774867421	11.20555012	6.669591159	10.66006223	6.685159322	9.642095113	5.586399151	12.11305285	7.274264552	10.12287051	5.210383388	11.86827226	7.133185111
96	12.87669135	4.981826167	12.86678418	4.998963506	12.06139193	3.725233035	13.69476915	5.65823885	12.72925089	5.005896456	12.24466922	4.659440642	14.38940678	5.717518026	11.6972445	3.958776803	14.55633471	5.850247166	9.99056288	5.948208966	11.16373164	6.909861731	9.489723021	5.328715834	11.0944463	6.769568726	10.88356823	6.953037533	10.34206744	6.003804489	12.12776226	7.452037611	10.09655246	5.151344564	11.94510346	7.098023501
97	12.84855531	4.987455034	12.88696081	4.988873824	12.17266178	3.726598874	13.72374494	5.658294418	12.74992377	4.961606608	12.36986414	4.679412937	14.22529594	5.720645269	11.83915365	4.060974053	14.7114179	5.886378602	10.16843526	5.929435089	11.0230899	6.588400218	10.29324288	5.879434729	11.41906468	6.90646486	10.55857648	6.758894435	10.41123869	5.881423597	12.00511686	7.241584716	10.09927329	5.128455482	11.8937937	7.041435213
98	12.80717929	4.962622799	12.87149292	5.018724418	12.25761721	3.799323796	13.64661545	5.629281428	12.74476994	4.997875106	12.31785785	4.680841168	14.36554878	5.695728875	11.70105761	4.001901022	14.63346328	5.903046552	10.0534816	5.760002893	10.99821033	6.468069841	10.09923681	5.653219898	11.38810347	6.95326475	10.91130146	6.745114218	10.47079569	6.063564137	11.96266084	7.10782425	10.32992803	5.272665698	11.8962924	6.994521163
99	12.8309349	4.973583706	12.86306794	5.018251869	12.18169358	3.799041799	13.72253436	5.630094887	12.78485204	4.999289698	12.3685345	4.631583888	14.42165012	5.695536978	11.66508052	3.966383244	14.65026611	5.852777532	10.04178921	5.920728529	10.91744658	6.588337503	9.911407564	5.662931773	11.23920568	6.849329622	10.53710815	6.813221998	10.20417159	5.757249281	11.75518586	6.595318051	10.02023245	5.22088422	11.83161686	7.0859147
100	12.84387964	4.956372754	12.82662445	4.983231975	12.30890584	3.801614943	13.65448367	5.575742619	12.71233976	5.040173112	12.45978168	4.634088864	14.3369057	5.723222724	11.73568001	3.968809259	14.58278254	5.871669529	9.660699256	5.609902281	11.05469866	6.745886432	9.920187402	5.683348511	11.21818382	6.869241549	10.6621287	6.886170945	9.979074526	5.554284647	12.17556855	7.485820295	10.14929728	5.355699796	12.04672636	7.3310702
101	12.83711395	4.955670721	12.83772388	5.000233637	12.12561941	3.768104678	13.64809862	5.583962115	12.76047042	4.983596321	12.11524732	4.634329405	14.35101432	5.746137806	11.5070257	3.940885347	14.61003411	5.863744417	9.902106387	5.691860914	11.04900227	6.513222062	10.04828783	5.842277963	11.24500279	6.613837505	10.84020042	6.806064816	10.38002169	5.863600611	12.06605149	7.144785589	10.17243189	5.297330978	11.78636785	6.932958311
102	12.83624563	4.964781784	12.87475633	4.985842027	12.21105134	3.831872844	13.64996877	5.601439466	12.78381106	5.027078419	12.34633228	4.615529502	14.35764253	5.708370307	11.69594921	3.976080138	14.59947489	5.87729733	9.726509622	5.575710983	10.98177034	6.466559492	10.11090947	5.76702938	11.27872836	6.714759409	10.98472993	6.928928476	10.24860602	5.855968129	11.87964826	6.937035874	10.15890056	5.277466302	12.0274949	7.310875475
103	12.81031644	5.002835599	12.89526243	5.003969721	12.28418042	3.809772913	13.71294234	5.588856294	12.83057137	5.019988277	12.24997105	4.579333401	14.37347652	5.699791199	11.79131692	4.011093685	14.61795689	5.869432632	10.10551516	5.93652109	10.95488438	6.564453975	9.937749946	5.702519247	11.16408885	6.667561673	10.77347903	6.93445261	10.21641315	5.958245434	11.96643142	7.291690287	10.05427673	5.221815471	11.86612985	7.100281039
104	12.79837515	4.97577179	12.89013346	4.974404142	12.24703831	3.814839984	13.67837343	5.582152607	12.80445694	4.965488243	12.33803932	4.610180247	14.38062101	5.709759422	11.66876293	3.94912358	14.52360425	5.862025044	10.2499466	5.884198131	11.03753298	6.710724171	10.49374771	5.985316834	11.40492174	6.841429583	10.79924093	6.773188027	10.22015012	5.960472141	11.89131551	7.039946479	9.779037436	5.152039106	11.87885867	7.081630041
105	12.81266046	4.950350493	12.8793587	4.978364566	12.20432431	3.769067859	13.67042015	5.581281554	12.77522444	5.003038798	12.42791069	4.633625991	14.36991529	5.720639842	11.40675577	3.94370049	14.64653602	5.865059183	10.23957582	5.939544723	10.95748279	6.630674213	10.58210059	6.117432192	11.32076078	6.716112998	11.04622494	6.928904919	10.1465125	5.804934006	11.99796019	7.149061868	9.894235356	5.094900399	11.93157801	7.358265064
106	12.83886331	4.942494164	12.84272497	4.981927755	12.26183397	3.7755718	13.66423723	5.553971996	12.82773448	5.075115935	12.58997764	4.627509357	14.38781466	5.710858959	11.67891943	3.968281065	14.63230033	5.855723214	10.2461883	5.790572959	10.99918466	6.67947722	10.0306269	5.741543347	11.1660243	6.668973199	10.77193343	6.889762755	9.970902147	5.688996866	12.22933332	7.230819681	10.29518884	5.468879781	11.73426148	6.845561762
107	12.80283575	4.90724945	12.8593807	4.953368522	12.25314126	3.820571891	13.65539955	5.60549172	12.81655979	5.033085097	12.4217274	4.632623724	14.3658585	5.716473199	11.62661517	3.964112358	14.53729081	5.868179856	10.12061045	5.785430149	11.12193179	6.905210276	10.21183344	5.70742428	11.42108936	6.876441013	10.78613974	6.749377017	10.71833156	6.179806508	12.12931734	7.237600502	10.24676747	5.361106922	11.87695388	7.27480036
108	12.71768544	4.943276771	12.86021344	4.969464033	12.2314715	3.841364801	13.66250316	5.617166314	12.77191421	5.037208917	12.48353148	4.64421144	14.30659588	5.712457712	11.55540365	3.978042877	14.54642596	5.865417132	10.01077254	5.809250353	11.11532656	6.720996845	10.05036616	5.683794179	11.35956909	6.75084894	10.80517681	6.717454902	10.45076582	5.958831846	12.19909926	7.321310871	10.28763789	5.578689921	11.71241604	7.150368794
109	12.84858802	4.925710226	12.88076753	4.966292372	12.31282081	3.803625176	13.64670372	5.597022104	12.88262889	5.0682246	12.36007645	4.631940896	14.32438326	5.703031739	11.76531521	3.956412991	14.66941544	5.869425391	9.677457885	5.522766977	10.83207925	6.502647875	10.13908717	5.884730662	11.40230476	6.986101941	10.76765531	6.893298134	10.05606901	5.688785256	12.02238815	7.208448968	9.835734131	4.97511324	12.07893458	7.205221689
110	12.81071821	4.895165655	12.82334156	4.979711578	12.18820192	3.857288581	13.71087624	5.546044616	12.72073126	5.013360796	12.23790726	4.64190626	14.30356509	5.682885803	11.58129231	3.970350659	14.62410179	5.871518676	9.997073321	5.902477807	11.06474782	6.701498418	10.6595285	5.994966572	11.4791537	6.897468397	10.59578032	6.59549818	10.12966215	5.70221501	11.93660336	6.978948775	10.24841281	5.354727432	11.95041203	6.987774556
111	12.81990573	4.929075605	12.86304803	4.930234077	12.2152533	3.793818751	13.65558411	5.56888326	12.80591144	5.010172442	12.23239733	4.612961951	14.33566498	5.713310235	11.65699524	3.973848643	14.61796316	5.879149942	9.704490054	5.554307747	10.91806593	6.580170524	9.777917554	5.558908149	11.18740679	6.68478289	10.4866192	6.72227732	9.899601242	5.736448178	12.16019721	7.252632902	10.5401546	5.721868126	11.99237512	7.039882232
112	12.81422952	4.90657001	12.83806789	4.96289112	12.08988419	3.775748426	13.66978632	5.584313383	12.81187123	5.043329189	12.29478273	4.577300097	14.35951533	5.69389276	11.61611063	3.980343814	14.55053585	5.866327335	9.737589498	5.432794349	11.22760631	6.815386605	10.04125532	5.811587239	11.18357637	6.565915758	10.58663629	6.910537117	10.16555647	5.930055674	12.00226855	7.122440692	10.07464	5.281867192	12.04979677	7.296073545
113	12.82403054	4.942121114	12.82966147	4.949896315	12.14954805	3.786545169	13.67778978	5.566631093	12.89060832	5.027338521	12.40393968	4.658333824	14.31064617	5.680632794	11.68674117	3.937318407	14.55052088	5.844503697	10.04133527	5.754796624	11.0943575	6.670542071	10.3314148	5.885479719	11.46594067	6.988184827	10.75736728	6.670980281	10.02475737	5.70962378	12.05953413	7.12553383	10.09123549	5.242732444	11.74944364	7.096877582
114	12.79330061	4.917801484	12.86371095	4.946130531	12.17135	3.812670796	13.69080071	5.589003677	12.83605396	4.988604121	12.36678313	4.646549653	14.33949265	5.70151645	11.63839464	3.943821539	14.60918145	5.866194287	10.34377667	5.972377426	11.05878627	6.644295556	10.1998275	5.974013763	11.05757197	6.576478601	10.70614271	6.730935399	9.841425313	5.57704384	12.117765	7.30376679	10.12147153	5.28524629	11.90333261	7.269870574
115	12.82969355	4.941428381	12.82450664	4.963071378	12.24720999	3.800911595	13.68150261	5.568327451	12.8348799	5.03415172	12.13159748	4.561730671	14.36644579	5.65463245	11.60853214	3.950616252	14.63424336	5.862911693	9.50292255	5.580824178	11.07461591	6.660209361	9.825421655	5.7887027	11.46195239	6.872655181	10.91060616	6.907220499	10.34103256	5.913363843	12.15466745	7.230947494	9.912032456	5.119475416	11.81852905	7.160600122
116	12.8344274	4.95237517	12.83603483	4.985768088	12.19969076	3.836259387	13.67827677	5.5853665	12.83353795	5.012210337	12.06866848	4.633961672	14.32353522	5.664097228	11.4047413	3.940069616	14.53952583	5.88465433	10.29245894	5.922649965	11.06022308	6.69568476	10.09465684	5.893621911	11.4307837	7.035501862	10.52709106	6.746999411	10.27194515	5.899114724	11.89012425	7.043608325	10.406114	5.431057489	11.76378572	7.033628057
117	12.81662182	4.882155658	12.82300643	4.94854762	12.22415791	3.7911523	13.68418953	5.610803459	12.8785162	5.051245267	12.26394598	4.587029897	14.32010825	5.689907178	11.49760103	3.85467016	14.50243632	5.848284408	10.23147504	5.900971292	11.16872159	6.716601693	10.05775836	5.878897703	11.17189934	6.638618053	10.66849893	6.811427496	10.18496121	5.755273919	11.91420674	6.924533248	10.39601831	5.46663975	11.94251754	7.127765457
118	12.83567654	4.896398841	12.88516008	4.957256255	12.18229973	3.781432773	13.7011324	5.583397466	12.68563044	5.000911536	12.28435638	4.64808654	14.3326722	5.689249956	11.51875592	3.946413328	14.68485556	5.846390275	9.894078548	5.701044967	10.89144082	6.400621653	10.48625786	6.051698781	11.10570677	6.617005619	10.85989842	6.869862507	10.03893056	5.613618333	12.15343061	7.154006864	10.07488259	5.168476184	11.76449642	6.910695834
119	12.81175649	4.943958961	12.82071379	4.925456356	12.12193055	3.781566725	13.63176514	5.546800848	12.83794573	5.081783045	12.18576446	4.601711178	14.33815669	5.660453522	11.69185347	3.960616294	14.61681592	5.885256783	9.738188953	5.477127767	10.98860376	6.567630022	10.06757669	5.671078927	11.3881473	6.911681484	10.64980622	6.7763501	10.03490893	5.937888667	12.10467383	7.198875966	10.25884257	5.418465144	11.75041914	7.011412101
120	12.83325104	4.94740682	12.83010836	4.953002206	12.10269992	3.768087328	13.67356026	5.568314758	12.71298985	5.029456534	12.18441702	4.639483502	14.31077708	5.668127335	11.65913145	3.925773813	14.51526925	5.869011912	9.901676202	5.769269346	10.92923034	6.528280597	9.879061429	5.600154242	11.19573068	6.654367328	10.6616172	6.965508472	10.29229594	5.852807274	12.17225793	7.379385973	10.23063001	5.47208894	11.79183187	7.058394956
121	12.79838543	4.889203176	12.82825464	4.948291373	12.19185095	3.804720418	13.64550938	5.565988453	12.78730386	5.092991192	12.19445081	4.596457615	14.33644463	5.688906113	11.75825443	4.026918986	14.56076353	5.864007654	10.07292496	5.896254684	11.11344299	6.73734606	9.800108021	5.583137518	11.27409779	6.748548381	10.59185646	6.845784936	10.45974718	6.011544505	12.24104252	7.25126723	10.20817607	5.36957483	11.84445131	6.778445452
122	12.79717803	4.888045908	12.81560677	4.937239596	12.25348364	3.817450064	13.68190441	5.585509129	12.75269834	5.012801703	12.3231117	4.672323067	14.37268415	5.673005271	11.57837433	3.969432276	14.58516659	5.848770808	10.07855144	5.922102049	10.97636295	6.627284113	9.816816115	5.616825287	11.23468566	6.720678812	10.7484782	6.842816078	9.967817264	5.860221959	12.09168116	7.416095123	10.31241593	5.457029526	11.89870299	7.119764539
123	12.82813017	4.90081477	12.80783892	4.914751412	12.15591701	3.782718095	13.6806986	5.557735472	12.80493283	5.022681173	12.36693484	4.658119919	14.3866263	5.667857444	11.62412494	3.90694604	14.48959351	5.814751347	10.16467191	5.821406353	10.88627698	6.441823451	10.12154574	5.849506107	11.44053393	6.955696429	10.87169657	6.936549585	10.11828478	5.76940784	12.11837951	7.355881283	9.987438406	5.176661876	11.86098847	7.099480647
124	12.79662914	4.948221825	12.84193393	4.939008795	12.11954941	3.759706887	13.65843646	5.551023721	12.8074663	4.977573942	12.35049794	4.667091637	14.34833524	5.689064327	11.46539558	3.942910481	14.6331364	5.847765346	9.848707268	5.84248759	10.85331314	6.51128046	9.730691598	5.559652844	11.27695766	6.912326286	11.17374909	7.280397085	10.12036371	5.806908499	12.08545963	7.423253814	9.914081754	5.175746251	11.79850869	7.053699823
125	12.78990301	4.888755386	12.79586732	4.93818904	12.23031746	3.761291639	13.61837504	5.553101896	12.80761572	5.018312623	12.57411856	4.644537004	14.29446151	5.682931424	11.57584992	3.996922926	14.61003227	5.836853476	9.727297552	5.63630544	11.01454642	6.630280703	10.30185864	5.782668469	11.43942606	6.877975648	10.38224069	6.739827713	10.09366126	5.89637832	12.28915171	7.555787934	10.20403803	5.359303217	11.86365993	7.047219841
126	12.74868521	4.835843281	12.84477743	4.943975399	12.19927664	3.783458677	13.67055755	5.570781835	12.84530883	5.033835086	12.37608949	4.690994898	14.28013398	5.670162447	11.64691264	3.942536156	14.60359262	5.869739168	9.707125704	5.557860325	11.14700091	6.665945051	9.821498414	5.420158962	11.33428596	6.873392099	10.73198057	6.653888762	9.876565162	5.820436933	12.19745116	7.345003989	9.834641185	5.088305185	11.82473976	7.229893274
127	12.79771759	4.897847326	12.84279102	4.942595456	12.11806005	3.778000652	13.70510531	5.546024177	12.82263613	5.04821126	12.46151046	4.710558425	14.28862508	5.673389426	11.8296278	4.02090872	14.62363919	5.8607223	9.934737944	5.748342399	11.04809929	6.636630784	9.824356626	5.54765088	11.00521485	6.394178047	10.79771139	6.750663741	10.04102135	5.718080738	12.27696247	7.55500509	10.42149043	5.54377483	12.1709476	7.639188766
128	12.78111358	4.910827203	12.84023354	4.928884111	12.16354128	3.790360462	13.64150315	5.56281142	12.85735462	5.038504079	12.10938637	4.636901062	14.35361012	5.679128892	11.42142457	3.920642141	14.65294816	5.861282281	10.08549763	5.850191634	11.09367498	6.68095709	10.53846282	6.097791589	11.25537554	6.637050626	10.75183213	6.803631852	10.38655331	5.790427494	12.01411433	7.229158158	10.07102069	5.117999218	11.84551709	6.865543967
129	12.76654309	4.873207613	12.82133503	4.94570242	12.14858148	3.810218113	13.69022995	5.535903119	12.91815151	5.027773593	12.39892089	4.64027941	14.27846364	5.674354456	11.5352307	3.945425653	14.56377491	5.881108146	9.85688747	5.719847254	11.23945742	6.682259258	10.02107866	5.714732008	11.14764308	6.657733711	11.03177825	6.921678021	10.19717532	5.755950231	12.08073399	7.387147189	10.52565228	5.558222078	11.77278566	6.782902263
130	12.80508521	4.918298793	12.8198493	4.917314498	12.04618411	3.778427861	13.69357358	5.531458389	12.79094375	5.035313306	12.15317128	4.674355006	14.34125959	5.669136123	11.44598586	3.946659318	14.68441689	5.857853675	9.868370241	5.772052277	10.97321292	6.370856372	9.910701528	5.495370781	11.11818588	6.545146123	10.80328438	6.939126642	10.00290194	5.86370115	12.06405765	7.331804734	9.940267144	5.091374841	11.8490186	6.787229955
131	12.78004285	4.902656796	12.82602271	4.908297357	12.1914132	3.850868529	13.69590659	5.535858688	12.81917907	5.04576403	12.31492329	4.687655208	14.3182015	5.702833336	11.38103331	3.907597226	14.59082497	5.859602499	9.880833884	5.782558578	10.99217033	6.645265199	9.918542537	5.582013117	11.30359613	6.730429088	10.86625414	6.890134231	9.896071348	5.486964212	12.09802109	7.218212324	9.926925202	5.163742183	11.76805876	6.881117052
132	12.74921131	4.848417253	12.84359716	4.922805329	12.17153835	3.799522307	13.71647376	5.576125593	12.87355118	5.021974269	12.4026007	4.635488998	14.2448143	5.669131173	11.61569033	3.935526001	14.55935445	5.82823116	9.768652724	5.549645844	11.00480444	6.506151212	10.40003871	6.066178953	11.21716308	6.748367113	10.86921572	6.774250947	10.05133016	5.881188506	12.05140918	7.062161245	10.16477984	5.355758829	11.91472765	7.06387726
133	12.83534881	4.902909889	12.8250919	4.9426671	12.23736958	3.84578446	13.69633623	5.564114724	12.69747012	5.026082268	12.41614214	4.634222323	14.32886073	5.682574897	11.71861241	3.980710482	14.65712689	5.830498993	10.00202282	5.697725873	10.92085286	6.538024992	10.01963683	5.905156891	11.19376276	6.64735251	10.61226602	6.863780977	9.932145262	5.603386974	12.24802091	7.513062354	10.42548601	5.428112489	11.84696015	7.108834986
134	12.75154784	4.877172741	12.80268344	4.930260543	12.24798816	3.840231778	13.70233814	5.556934404	12.82346575	5.038906009	12.3670005	4.655576255	14.34473152	5.639698328	11.50079864	3.955520338	14.65610936	5.844849428	9.884723068	5.758619053	11.1628503	6.943305947	10.15865289	5.786828869	11.37713891	6.837691218	10.72000068	6.884633286	10.13839481	5.70756129	11.92051026	6.978863924	10.23576969	5.372940561	11.69646741	6.789677687
135	12.78700085	4.874019412	12.79370593	4.887559953	12.11337185	3.777217606	13.69895679	5.555501768	12.93332079	5.061476114	12.32262688	4.689543777	14.35588021	5.685032768	11.59255752	3.972989566	14.64151506	5.83930194	9.770105323	5.78337825	10.84146317	6.658866839	10.16255807	5.964378028	11.3461214	6.823808283	10.74485662	6.816553147	10.17183397	5.783931863	12.17506336	7.286251563	10.02621106	5.265071582	12.19012729	7.307736187
136	12.77824402	4.842295044	12.81165296	4.912589946	12.18825773	3.833206517	13.66359206	5.552033828	12.75319352	5.030336162	12.27834098	4.659722508	14.29480551	5.642606268	11.49623944	3.925651125	14.63473802	5.827168074	9.770033619	5.663976594	11.04738505	6.660766987	9.824477391	5.527542791	11.22238761	6.679542487	10.76924983	6.90060686	9.936587037	5.617458785	12.13747755	7.217363432	9.979296071	5.26790927	12.04324895	7.261427526
137	12.80113956	4.856931927	12.79600039	4.925958078	12.24114671	3.805372584	13.66441478	5.549537231	12.77772333	5.041782907	12.29186868	4.667493253	14.36013254	5.683753209	11.66880799	3.957783283	14.59761366	5.817835149	9.745606396	5.605960766	11.06312429	6.721946514	9.870089044	5.533901152	11.31656378	6.85199684	10.56840209	6.84180023	9.846836317	5.600624902	12.09073464	7.355920142	10.03173085	5.304818519	11.81102873	6.960800308
138	12.78244214	4.836770196	12.84578378	4.92634531	12.22054422	3.811827157	13.64962732	5.54863981	12.87364091	5.021672571	12.32598817	4.659993484	14.35941424	5.662380972	11.83809669	3.984635697	14.58653201	5.83446761	10.0488913	5.823370062	10.89081424	6.362107241	9.973957703	5.725082545	11.33668507	6.829489128	10.99156405	7.068413876	10.07000738	5.640983261	12.07935016	7.154672489	10.40185319	5.488853602	11.84783403	7.104098691
139	12.75987641	4.86861335	12.81700101	4.888208975	12.20323539	3.761631776	13.64429982	5.520231773	12.86211157	5.000035966	12.42168211	4.660172772	14.3279671	5.640176131	11.63184752	3.946291024	14.55779328	5.841923619	9.743344436	5.678929647	10.98147676	6.586991692	10.05290527	5.649536571	11.16616225	6.650951765	10.66299231	6.907943713	10.25103984	5.833822782	12.27417684	7.72552562	10.44004542	5.483166528	11.91187052	7.081602355
140	12.76733847	4.843614296	12.80926754	4.866934769	12.20607693	3.790103632	13.65827168	5.527433256	12.80038719	5.027811256	12.26042732	4.64514514	14.33426781	5.674531874	11.44451555	3.955196457	14.62456373	5.820214272	9.842470134	5.683358988	11.09408297	6.54438041	9.907908691	5.657234337	11.37192611	6.918745303	10.7050342	6.724597227	9.954471682	5.723080484	11.95071227	6.86998938	10.17596332	5.389509533	11.74279243	7.100379571
141	12.79871619	4.920151338	12.81793416	4.868528538	12.29118095	3.834812176	13.60366588	5.534938856	12.70751072	5.039065317	12.45575443	4.610145484	14.30119041	5.681262365	11.34552543	3.906217435	14.59454989	5.85626637	9.976902412	5.877481409	10.8600229	6.430590816	10.13936719	5.838635235	11.36050424	6.72967497	10.9619546	7.009913003	10.30434766	5.895999352	11.87440855	6.846996908	10.34758993	5.323956957	12.00189086	7.181353087
142	12.8212466	4.889768083	12.78111864	4.888541127	12.14109127	3.811559718	13.69329994	5.547905787	12.79553513	5.033195939	12.55525663	4.691394817	14.3036459	5.668863621	11.54666539	3.959354476	14.63987291	5.838204069	10.04600649	5.956972756	10.91387071	6.517014613	10.30588664	5.988598373	11.24879302	6.66591785	10.40134575	6.63073466	10.08082029	5.867580169	12.10802299	7.046684768	10.38011485	5.552064577	11.87875927	6.959758573
143	12.7476677	4.84813491	12.80644969	4.882378646	12.08598273	3.813090725	13.63670087	5.526719529	12.85525979	5.05823895	12.39350875	4.650321618	14.35320895	5.692755004	11.51312146	3.944838708	14.57761688	5.859457008	9.831028463	5.685965255	11.04069617	6.67873601	10.1945014	5.900027948	11.21202515	6.828127923	10.55561956	6.783316077	9.861167779	5.609331582	11.99798826	7.308597833	10.04516952	5.250026663	11.84555263	6.962079633
144	12.79322758	4.876993729	12.82238409	4.892348759	12.20387987	3.848930161	13.73174927	5.536782187	12.84785623	5.03198613	12.34290919	4.648853902	14.35478183	5.679136748	11.80573735	3.949575896	14.57032419	5.837159597	9.888221996	5.809498725	11.05911924	6.550454252	10.00606877	5.926501886	11.10807344	6.543029917	10.89384118	6.914599864	10.13868618	5.787697775	12.14466068	7.219994004	10.39483916	5.387116397	11.80479644	7.103919914
145	12.7285103	4.859770938	12.84004603	4.854653157	12.21097069	3.846971694	13.66409641	5.523727082	12.94570186	5.033022252	12.35886178	4.694104644	14.33969617	5.675255397	11.32528397	3.874822784	14.55463792	5.834215761	9.618667864	5.583314574	10.9861388	6.444298454	9.802548669	5.586639358	11.32165164	6.653080209	10.60808077	6.73660428	10.23741471	5.867470837	12.18748199	7.559728022	10.45188947	5.763574802	11.74657201	6.969316147
146	12.80325616	4.875210542	12.77451206	4.89549781	12.14096706	3.813878993	13.68018965	5.478006944	12.76117529	5.055495521	12.41700791	4.682381889	14.33002258	5.6321648	11.35920882	3.869627152	14.63237197	5.827740488	10.07436561	5.748606989	10.98501656	6.575790436	10.36640201	6.067780017	11.33959427	6.786324814	10.75068956	6.792828863	10.3187113	5.907204748	12.04589084	7.211231636	9.905364463	5.174264432	11.88064427	7.386005324
147	12.79866765	4.877512288	12.7766732	4.865815006	12.11076059	3.782654137	13.66207769	5.505739502	12.91428586	5.058649514	12.3428018	4.652201193	14.37295143	5.646128018	11.67088383	3.950340902	14.56811404	5.868104738	10.14420386	6.033079216	10.96447246	6.69652029	10.22924903	5.956134482	11.22581853	6.687911685	11.12761843	7.04446295	9.88740362	5.735655627	11.96795116	7.054176644	10.45206561	5.481307353	11.80802661	6.831936088
148	12.78318758	4.830364874	12.79500604	4.866292152	12.28218445	3.819352235	13.63169277	5.51955701	12.79222164	5.017478271	12.48938048	4.683189679	14.35826719	5.668358137	11.54615244	3.85040248	14.61391602	5.846942853	10.12216864	5.830985206	11.00426196	6.599183805	9.839670328	5.8333683	11.31409282	6.769288706	10.7986547	6.919060987	10.30780409	5.901554566	12.23929732	7.406138587	10.28687581	5.428033398	11.92732853	7.157971781
149	12.8187729	4.87035144	12.82313655	4.877171437	12.19801728	3.880430545	13.66471337	5.502911062	12.80986027	5.038513272	12.22711035	4.643707502	14.32660649	5.653893441	11.61600216	3.885628273	14.48555092	5.806691696	9.791636868	5.509685698	10.88996303	6.515683279	9.974603953	5.785849465	11.31518779	6.902047374	10.94955515	6.829147143	10.16443155	5.772992801	12.15883224	7.311724277	9.683102775	4.950058482	12.05349174	7.073306543
150	12.85246204	4.863471576	12.81484394	4.854252699	12.17277746	3.822648104	13.67699868	5.517687273	12.79299416	5.006378613	12.52068116	4.677390604	14.3256483	5.644663014	11.58464392	3.909713347	14.49338424	5.821866468	9.305453923	5.576061465	10.66488064	6.635259604	9.272655812	5.557183919	10.87474959	6.823608926	9.579883606	6.601194252	9.098271658	5.420294203	11.60686437	7.260848958	9.401739254	5.014099623	11.54042359	7.214859133
151	12.77586085	4.827727909	12.79027293	4.836292735	12.22258739	3.820553448	13.63592279	5.507602742	12.79830981	4.993104257	12.78807302	4.703038569	14.30159948	5.623623431	11.40294054	3.926377376	14.60834329	5.844616761	9.28774266	5.668098855	10.83810715	6.748001081	9.378289636	5.719660755	11.04365394	7.020838147	9.55864366	6.698941317	8.909183133	5.491625611	11.68757373	7.314993256	9.429714863	5.000042608	11.66461281	7.351882163
152	12.78760499	4.827192428	12.77960461	4.821843199	12.28056445	3.811450454	13.6349606	5.506521862	12.75763214	5.077481512	12.28154698	4.653277678	14.29384411	5.671385424	11.55941329	3.938968634	14.50943653	5.855551474	9.431565976	5.780264332	10.95821487	6.937421574	9.521267179	5.86508887	11.17486601	7.18010629	9.768143185	6.829481289	9.250055962	5.57525481	11.7845613	7.389228177	9.606675788	5.148617859	11.78347111	7.483418856
153	12.80903987	4.881625772	12.80355834	4.861209469	12.28135953	3.89364558	13.68388457	5.52702079	12.75047884	5.008270826	12.45756833	4.702262875	14.30521377	5.6484279	11.57464634	3.939112706	14.5967718	5.820314006	9.517301664	5.894862764	11.05116937	7.048892192	9.65949839	5.882536258	11.30430297	7.296427638	9.862130171	6.86487018	9.383388279	5.706456417	11.83803116	7.360245752	9.673938425	5.249028745	11.90414157	7.53506995
154	12.7269386	4.824986169	12.76898817	4.856126791	12.25619874	3.843670397	13.63779752	5.52516692	12.8262222	5.026919017	12.16776635	4.657794572	14.37053739	5.668802708	11.67359032	3.941861498	14.54439177	5.831566474	9.562466378	5.957363278	11.18391242	7.162174786	9.79514999	5.937555266	11.42279183	7.448460447	9.92021829	6.892418706	9.424195301	5.735555683	11.87960888	7.394470141	9.85667895	5.294111471	11.99393746	7.596119175
155	12.77489869	4.910327637	12.79184398	4.853732059	12.2393929	3.832542025	13.61294221	5.489050729	12.78271346	5.051922832	12.51833437	4.641307962	14.37234443	5.646842516	11.34075659	3.892330484	14.6199467	5.814788012	9.638230243	5.994404656	11.19605174	7.220280495	9.759444753	6.069157264	11.5695266	7.530846112	9.987719377	6.997165465	9.380408019	5.780297068	11.96332141	7.402533058	9.813137752	5.346177321	12.01415396	7.633758585
156	12.72258846	4.855299585	12.83263687	4.873767168	12.10208423	3.831572285	13.67187407	5.512221107	12.82279353	5.050845496	12.41500427	4.694633329	14.36008013	5.665114057	11.54142024	3.939545361	14.55725667	5.822363547	9.7883519	6.10474418	11.34331951	7.292956671	10.08219483	6.161312318	11.66851242	7.710974723	10.08791557	7.070545974	9.82516716	5.938164851	11.99142418	7.401492828	10.129105	5.524474258	12.11537185	7.665266117
157	12.77273829	4.878179146	12.76670855	4.838604918	12.17916072	3.787443829	13.65224755	5.515389647	12.79963995	5.048960832	12.18944835	4.663012894	14.36369228	5.648509545	11.42373148	3.881438983	14.59012224	5.82910544	9.778259168	6.157595486	11.37916423	7.393746385	10.09959771	6.216696957	11.70598826	7.679203964	10.26777989	7.124312502	9.661781208	5.961887807	12.02908206	7.398104354	9.957274274	5.579092142	12.24066084	7.685923535
158	12.72196537	4.819143381	12.78832409	4.869521577	12.37506133	3.827782379	13.66455005	5.51119294	12.80445471	5.046650768	12.20757285	4.656097748	14.29809053	5.658395727	11.74753105	3.92263164	14.6001415	5.835751559	9.955076815	6.265925481	11.49368657	7.466126236	10.18170322	6.264473446	11.84670146	7.921976285	10.28012648	7.190529001	9.84771074	6.05418479	12.03480248	7.38613601	10.33896463	5.654111607	12.25387516	7.705211968
159	12.74899657	4.837763836	12.83316595	4.857795888	12.22582603	3.828644756	13.68069863	5.502992268	12.89759237	5.06566595	12.29075264	4.653510869	14.28720767	5.651928143	11.76494106	3.976243098	14.55153336	5.79980272	9.958879264	6.282950842	11.55997723	7.625517372	10.33395533	6.356734568	11.96236448	7.978755914	10.43450948	7.218768574	9.938461133	6.095622016	12.12997924	7.389041223	10.23500471	5.69501962	12.32673228	7.737970645
